# Supplementary material for: The Geometry of Reachability in Continuous Vector Addition Systems with States
Source: arXiv:2210.00785 source file (2022-11-14)
Supplement: Supplementary file 1 [file appendix.tex]

\section{The interior of a convex cone is open}

Now, we prove that for any convex cone $C$ with basis $B$ it holds that $C \setminus \bound(B)$ is an open set. Usually, boundaries for convex cones are defined by the half-spaces of which the cone is an intersection. Whether the cone is open or closed depends on whether the half-spaces are open or closed. We prove this directly for our definition of boundary.

\begin{proof}
    To prove that $C\setminus \bound(B)$ is an open set, we will prove that every point $\vec{c}\in C\setminus\bound(B)$ has a neighbourhood. More formally, there exists $\varepsilon \in \mathbb{Q}_{>0}$ such that all points in a radius of $\varepsilon$ around $\vec{c}$ (with respect to the Euclidean distance) are also in $C\setminus\bound(B)$. 
    
    By definition of boundary, we know that there exist $\vec{v_1}, \vec{v_2} \in C$ such that $\vec{c} = \vec{v_1} + \vec{v_2}$ and $\vec{v_1} \not \in \linspan(\vec{v_2})$. Since $\vec{c} = \vec{v_1} + \vec{v_2}$, we have that $ \vec{c} \in \cone(\{\vec{v_1}, \vec{v_2}\})$. Hence, there exist $a_1, a_2\in \mathbb{Q}_{\geq 0}$ such that $\vec{c}$ is in the convex hull of $H \coloneqq \{\vec{0}, a_1\vec{v_1}, a_2\vec{v_2}\}$. Also, we know that $\vec{c} \not\in \cone(a_1\vec{v_1})$ and $\vec{c} \not\in \cone(a_2\vec{v_2})$ --- lest we contradict the fact that $\vec{v_1}$ and $\vec{v_2}$ are linearly independent. By choosing $a_1,a_2 > 1$ we can further assume that $\vec{c}$ is in the open convex hull of $H$. 
    By convexity, we have that all points in the convex hull of $H$ are also in $C$. Finally, since $\vec{c}$ has a neighbourhood in the convex hull of $H$, it does so too in $C$.
    
    \arkain{Since this is a simple fact, maybe we should give a more direct proof such as the following}
    
    Define the matrix
    \[
    \vec{A} =
    \begin{bmatrix}
    \vec{v}_1\\
    \vec{v}_2
    \end{bmatrix}
    \]
    Since $\vec{v}_1,\vec{v}_2$ are linearly independent,
    $\vec{A}$ is invertible.
    Define $f : \mathbb{Q}^2 \to \mathbb{Q}^2$ as
    \[
    f(\vec{u}) := \vec{A}^{-1}\vec{u}
    \]
    It follows that $f(\vec{u}) = (r,s)$ if and only if $\vec{u} = r \cdot \vec{v_1} + s \cdot \vec{v}_2$.
    This implies $f(\vec{v}) = (1,1)$.
    So $\vec{v} \in f^{-1}(\mathbb{Q}_{>0} \times \mathbb{Q}_{>0})$.
    $f$ is linear and hence a continuous function.
    Every vector $\vec{u} \in f^{-1}(\mathbb{Q}_{>0} \times \mathbb{Q}_{>0})$ can be written as $r \cdot \vec{v}_1 + s \cdot \vec{v}_2$ where $r,s > 0$.
    $r \cdot \vec{v}_1, s \cdot \vec{v}_2$ are linearly independent,
    so $\vec{u} \in (C \setminus \bound{(B)})$.
    Hence $f^{-1}(\mathbb{Q}_{>0} \times \mathbb{Q}_{>0}) \subseteq (C \setminus \bound{(B)})$.
    Therefore $f^{-1}(\mathbb{Q}_{>0} \times \mathbb{Q}_{>0})$ is an open set containing $\vec{v}$, inside $(C \setminus \bound{(B)})$.
    Since $\vec{v} \in (C \setminus \bound{(B)})$ was arbitrarily chosen,
    this implies for every $\vec{v} \in (C \setminus \bound{(B)})$ there is a open set $U_{\vec{v}} \subseteq C$ containing $\vec{v}$.
    Hence $(C \setminus \bound{(B)})$ is open.
    
\end{proof}

\section{Proof of \autoref{lemma:strictineq}}

Let $r \in \mathbb{Q}$. In this work, we suppose $r$ is given as a pair $p,q
\in \mathbb{Z}$ of integers encoded in binary. Further, we assume that $p$ and
$q$ are coprime. We write $\repr{r}$ to denote the number of bits required to
encode $p$ and $q$ in binary (disregarding the sign), that is $\repr{r}
\coloneqq \lceil \log_2(\abs{p} + \abs{q}) \rceil + 1$. For $\vec{v} \in
\mathbb{Q}^k$ we write $\repr{\vec{v}}$ for the sum $\sum_{i=1}^k
\repr{\vec{v}_i}$ and extend the notation to matrices
$\vec{A} \in \mathbb{Q}^{k \times \ell}$ by setting $\repr{\vec{A}}
\coloneqq \max_{i=1}^k \sum_{j=1}^\ell \repr{\vec{A}_{ij}}$.

From the work of Sontag we have the following result.
\begin{lemma}[From {\cite[Lemma 3.2]{sontag85}}]\label{lem:sontag}
    There exists a polynomial $f : \mathbb{N} \to \mathbb{N}$ such that, for
    all $\vec{A} \in \mathbb{Q}^{k \times n},\vec{C} \in \mathbb{Q}^{\ell
    \times n}$ and $\vec{b} \in \mathbb{Q}^k, \vec{d} \in \mathbb{Q}^\ell$,
    the system $\vec{Ax} \leq \vec{b} \land \vec{Cx} < \vec{d}$ has a solution
    if and only if it has a solution $\vec{a} \in \mathbb{Q}^n$ such that:
    \begin{equation}\label{eqn:bound}
      \repr{\vec{a}} \leq f(n)\repr{\begin{matrix}\vec{A} & \vec{b}\\
                                                   \vec{C} & \vec{d}\end{matrix}}.
    \end{equation}
\end{lemma}
Without loss of generality, we suppose the polynomial $f$ is monotone. Further, let us write $E$ to denote the right-hand side of \autoref{eqn:bound}. Then, $\vec{Ax} \leq \vec{b} \land \vec{Cx} < \vec{d}$ has a solution if and only if the following system has a solution:
\(
\vec{Ax} \leq \vec{b} \land \vec{Cx} \leq \vec{e}
\)
where, for all $i = 1, \dots, \ell$, we define
\(
    \vec{e}_{i} \coloneqq \vec{d}_i + 2^{-2(E^2)}.
\)

\begin{proof}[of \autoref{lemma:strictineq}]
    We prove the double implication mentioned above. That is, $\vec{Ax} \leq \vec{b} \land \vec{Cx} < \vec{d}$ has a solution if and only if the following system has a solution:
    \(
    \vec{Ax} \leq \vec{b} \land \vec{Cx} \leq \vec{e}.
    \)
    One direction is trivial. Indeed, any solution of the second system is also a solution of the original one. Below, we focus on solutions for the first system.
    
    Consider some $\vec{a} \in \mathbb{Q}^n$ that is a solution for the original system. We then have that $\vec{Ca} < \vec{d}$. We now establish an upper bound for $\repr{\vec{Ca}}$ based on \autoref{lem:sontag}. First, observe that:
    \begin{equation}\label{eqn:bound-c}
        \repr{\vec{C}}, \repr{\vec{d}} \leq \repr{\begin{matrix} \vec{A} & \vec{b}\\ \vec{C} & \vec{d} \end{matrix}}
    \end{equation}
    Let $i \in \{1, \dots, \ell\}$ be arbitrary. The following hold.
    \begin{align*}
        \repr{\vec{C}_i \vec{a}} ={} & \repr{\sum_{j=1}^n \vec{C}_{ij} \vec{a}_j}\\
        {} \leq {} & \repr{\prod_{j=1}^n \vec{C}_{ij} \vec{a}_j} & \text{by monotonicity of }\repr{\cdot}\\
        {} \leq {} & \sum_{j=1}^n \repr{\vec{C}_{ij}} + \repr{\vec{a}_j} & \log(xy) = \log(x) + \log(y)\\
        {} \leq {} & \sum_{j=1}^n \repr{\vec{C}_{ij}}\repr{\vec{a}_j}\\
        {} \leq {} & \sum_{j=1}^n \repr{\vec{C}_{i}}\repr{\vec{a}} & \text{monotonicity of } \max, +\\
        {} = {} & n \repr{\vec{C}_{i}}\repr{\vec{a}}+\\
        {} \leq {} & \left(f(n)\repr{\vec{C}_{i}}\repr{\vec{a}}\right)^2 & \text{by \autoref{lem:sontag}, \autoref{eqn:bound-c}}
    \end{align*}
    From the above inequalities and our initial assumption that $\vec{a}$ is a solution for the system (with strict inequalities) we know there are $p_1,p_2 \in \mathbb{Z}$ and $q_1,q_2 \in \mathbb{N}$ such that: 
    \[
      \vec{Ca} = \frac{p_1}{q_1} < \frac{p_2}{q_2} = \vec{d}_i
    \]
    and: 
    \[
        \log_2(\abs{p_1}),\log_2(\abs{p_2}),\log_2(\abs{q_1}),\log_2(\abs{q_2}) \leq E^2.
    \]
    This means that, $\varepsilon \coloneqq p_2/q_2 - p_1/q_1$ is a strictly positive value. Since $p_1,q_1,p_2,q_2$ are all integer, it follows that $\varepsilon \geq 1/(q_1q_2)$. From our bounds on the bits required to represent $q_1$ and $q_2$ we thus get that $\varepsilon \geq 2^{-2E^2}$ and that therefore $\vec{a}$ is also a solution of the second system.
\end{proof}
